# Supplementary material for: Scaling Graph-Based Dependency Parsing with Arc Vectorization and Attention-Based Refinement
Source: arXiv:2501.09451 source file (2025-01-16)
Supplement: Supplementary file 1 [file appendix_specialization_no_specialization.tex]

\begin{table*}[t]
\begin{adjustbox}{width=1\textwidth}
\small
\begin{tabular}{llrrll}
\toprule
\multicolumn{1}{c}{}         & Specialization & \multicolumn{1}{c}{\# Param ($10^{6}$)} & \multicolumn{1}{c}{Speed} & \multicolumn{1}{c}{UAS} & \multicolumn{1}{c}{LAS} \\ \hline
\multicolumn{6}{c}{PTB}                                                                                                                                                 \\
\textsc{Loc}                 & No             & 4                                       &                           &                         &                         \\
\textsc{Loc}                 & Yes            & 4                                       &                           &                         &                         \\
\textsc{CRF2o} projectivized & No             & 4                                       &                           &                         &                         \\
\textsc{CRF2o} projectivized & Yes            & 4                                       &                           &                         &                         \\
\textsc{ArcLoc} 0 layers     & No             & 4                                       &                           &                         &                         \\
\textsc{ArcLoc} 0 layers     & Yes            & 4                                       &                           &                         &                         \\
\textsc{ArcLoc} 1 layer      & No             & 4                                       &                           &                         &                         \\
\textsc{ArcLoc} 1 layer      & Yes            & 4                                       &                           &                         &                         \\
\textsc{ArcLoc} 2 layers     & No             & 4                                       &                           &                         &                         \\
\textsc{ArcLoc} 2 layers     & Yes            & 4                                       &                           &                         &                         \\
\hline
\textsc{Loc}                 & No             & 50                                      &                           &                         &                         \\
\textsc{Loc}                 & Yes            & 50                                      &                           &                         &                         \\
\textsc{CRF2o} projectivized & No             & 50                                      &                           &                         &                         \\
\textsc{CRF2o} projectivized & Yes            & 50                                      &                           &                         &                         \\
\textsc{ArcLoc} 0 layers     & No             & 50                                      &                           &                         &                         \\
\textsc{ArcLoc} 0 layers     & Yes            & 50                                      &                           &                         &                         \\
\textsc{ArcLoc} 1 layer      & No             & 50                                      &                           &                         &                         \\
\textsc{ArcLoc} 1 layer      & Yes            & 50                                      &                           &                         &                         \\
\textsc{ArcLoc} 2 layers     & No             & 50                                      &                           &                         &                         \\
\textsc{ArcLoc} 2 layers     & Yes            & 50                                      &                           &                         &                         \\
\hline
\multicolumn{6}{c}{UD}                                                                                                                                                  \\
\textsc{Loc}                 & No             & 4                                       &                           & 95.36                   & 93.47                   \\
\textsc{Loc}                 & Yes            & 4                                       & 497                       & 95.43                   & 93.57                   \\
\textsc{CRF2o} projectivized & No             & 4                                       &                           & 95.57                   & 93.62                   \\
\textsc{CRF2o} projectivized & Yes            & 4                                       & 162                       & 95.63                   & 93.69                   \\
\textsc{ArcLoc} 0 layers     & No             & 4                                       & 497                       & 95.30                   & 93.23                   \\
\textsc{ArcLoc} 0 layers     & Yes            & 4                                       & 484                       & 95.28                   & 93.25                   \\
\textsc{ArcLoc} 1 layer      & No             & 4                                       & 474                       & 95.38                   & 93.38                   \\
\textsc{ArcLoc} 1 layer      & Yes            & 4                                       & 450                       & 95.38                   & 93.40                   \\
\textsc{ArcLoc} 2 layers     & No             & 4                                       & 463                       & 95.29                   & 93.28                   \\
\textsc{ArcLoc} 2 layers     & Yes            & 4                                       & 448                       & 95.38                   & 93.40                   \\
\hline
\textsc{Loc}                 & No             & 50                                      & 456                       & 95.30                   & 93.42                   \\
\textsc{Loc}                 & Yes            & 50                                      & 463                       & 95.32                   & 93.44                   \\
\textsc{CRF2o} projectivized & No             & 50                                      & 116                       & 95.51                   & 93.55                   \\
\textsc{CRF2o} projectivized & Yes            & 50                                      & 159                       & 95.52                   & 93.56                   \\
\textsc{ArcLoc} 0 layers     & No             & 50                                      & 464                       & 95.48                   & 93.54                   \\
\textsc{ArcLoc} 0 layers     & Yes            & 50                                      & 459                       & 95.46                   & 93.53                   \\
\textsc{ArcLoc} 1 layer      & No             & 50                                      & 442                       & 95.58                   & 93.67                   \\
\textsc{ArcLoc} 1 layer      & Yes            & 50                                      & 421                       & 95.54                   & 93.66                   \\
\textsc{ArcLoc} 2 layers     & No             & 50                                      & 436                       & 95.57                   & 93.67                   \\
\textsc{ArcLoc} 2 layers     & Yes            & 50                                      & 419                       & 95.54                   & 93.66                   \\
\bottomrule
\end{tabular}
\end{adjustbox}
\caption{Dev LAS for the PTB and the averages of 12 languages in UD2.2.
}\label{tab:ud}

\end{table*}

%%% Local Variables:
%%% mode: latex
%%% TeX-master: "../main"
%%% End:
