# Supplementary material for: Scaling Graph-Based Dependency Parsing with Arc Vectorization and Attention-Based Refinement
Source: arXiv:2501.09451 source file (2025-01-16)
Supplement: Supplementary file 2 [file appendix_PTB_arc_sizes_comparison.tex]

\begin{table}[]
  \centering
  \small
%\begin{adjustbox}{width=0.49\textwidth}
\begin{tabular}{rrrrc}
\multicolumn{1}{l}{Word vector} & \multicolumn{1}{l}{Arc vector} & \multicolumn{1}{l}{Speed} & UAS            & \multicolumn{1}{r}{LAS} \\
\midrule
900                             & N/A (\textsc{Loc})             & 3xx                       & 96.85          & 95.16                   \\
70                              & 740                            & 3xx                       & 96.xx          & 95.xx                   \\
100                             & 380                            & 3xx                       & 96.xx          & 95.xx                   \\
130                             & 230                            & 3xx                       & 96.xx          & \textbf{95.xx}          \\
155                             & 160                            & 3xx                       & 96.xx          & 95.xx                   \\
180                             & 120                            & 3xx                       & \textbf{96.xx} & 95.xx                   \\
210                             & 85                             & 3xx                       & 96.xx          & 95.xx                   \\
240                             & 65                             & 3xx                       & 96.xx          & 95.xx
\end{tabular}
%\end{adjustbox}
\caption{PTB dev scores \wrt{} arc and word vector sizes (4M params) (8 run average, no transformer).}
\label{table:arc_sizes}
\end{table}

%%% Local Variables:
%%% mode: latex
%%% TeX-master: "../main"
%%% End:
